# Supplementary material for: Quantum Annealing based Feature Selection in Machine Learning
Source: arXiv:2411.19609 source file (2024-11-29)
Supplement: Supplementary file 1 [file 05-appendix.tex]

\section*{\uppercase{Appendix}}
\label{app:appendic}
